# Supplementary material for: DivAvatar: Diverse 3D Avatar Generation with a Single Prompt
Source: arXiv:2402.17292 source file (2024-02-27)
Supplement: Supplementary file 1 [file X_suppl.tex]

\clearpage
\setcounter{page}{1}
\maketitlesupplementary

This document provides supplementary materials in 1) additional qualitative comparisons, and 2) implementation details. More details to be found in the following subsections.

\section{Additional Qualitative Comparisons}
\label{sec:quali}
In this section, we provide additional examples on the qualitative comparisons between DivAvatar, Stable Dreamfusion, and AvatarCraft. For each prompt, we obtain five different samples for each method. The comparison is shown in \cref{fig:sweater,fig:green5,fig:shorts,fig:woman} below. Our method demonstrates significantly higher level of diversity as compared to Stable Dreamfusion and AvatarCraft.

\begin{figure*}[h!]
  \centering
  % \fbox{\rule{0pt}{2in} \rule{0.9\linewidth}{0pt}}
   \includegraphics[width=0.8\linewidth]{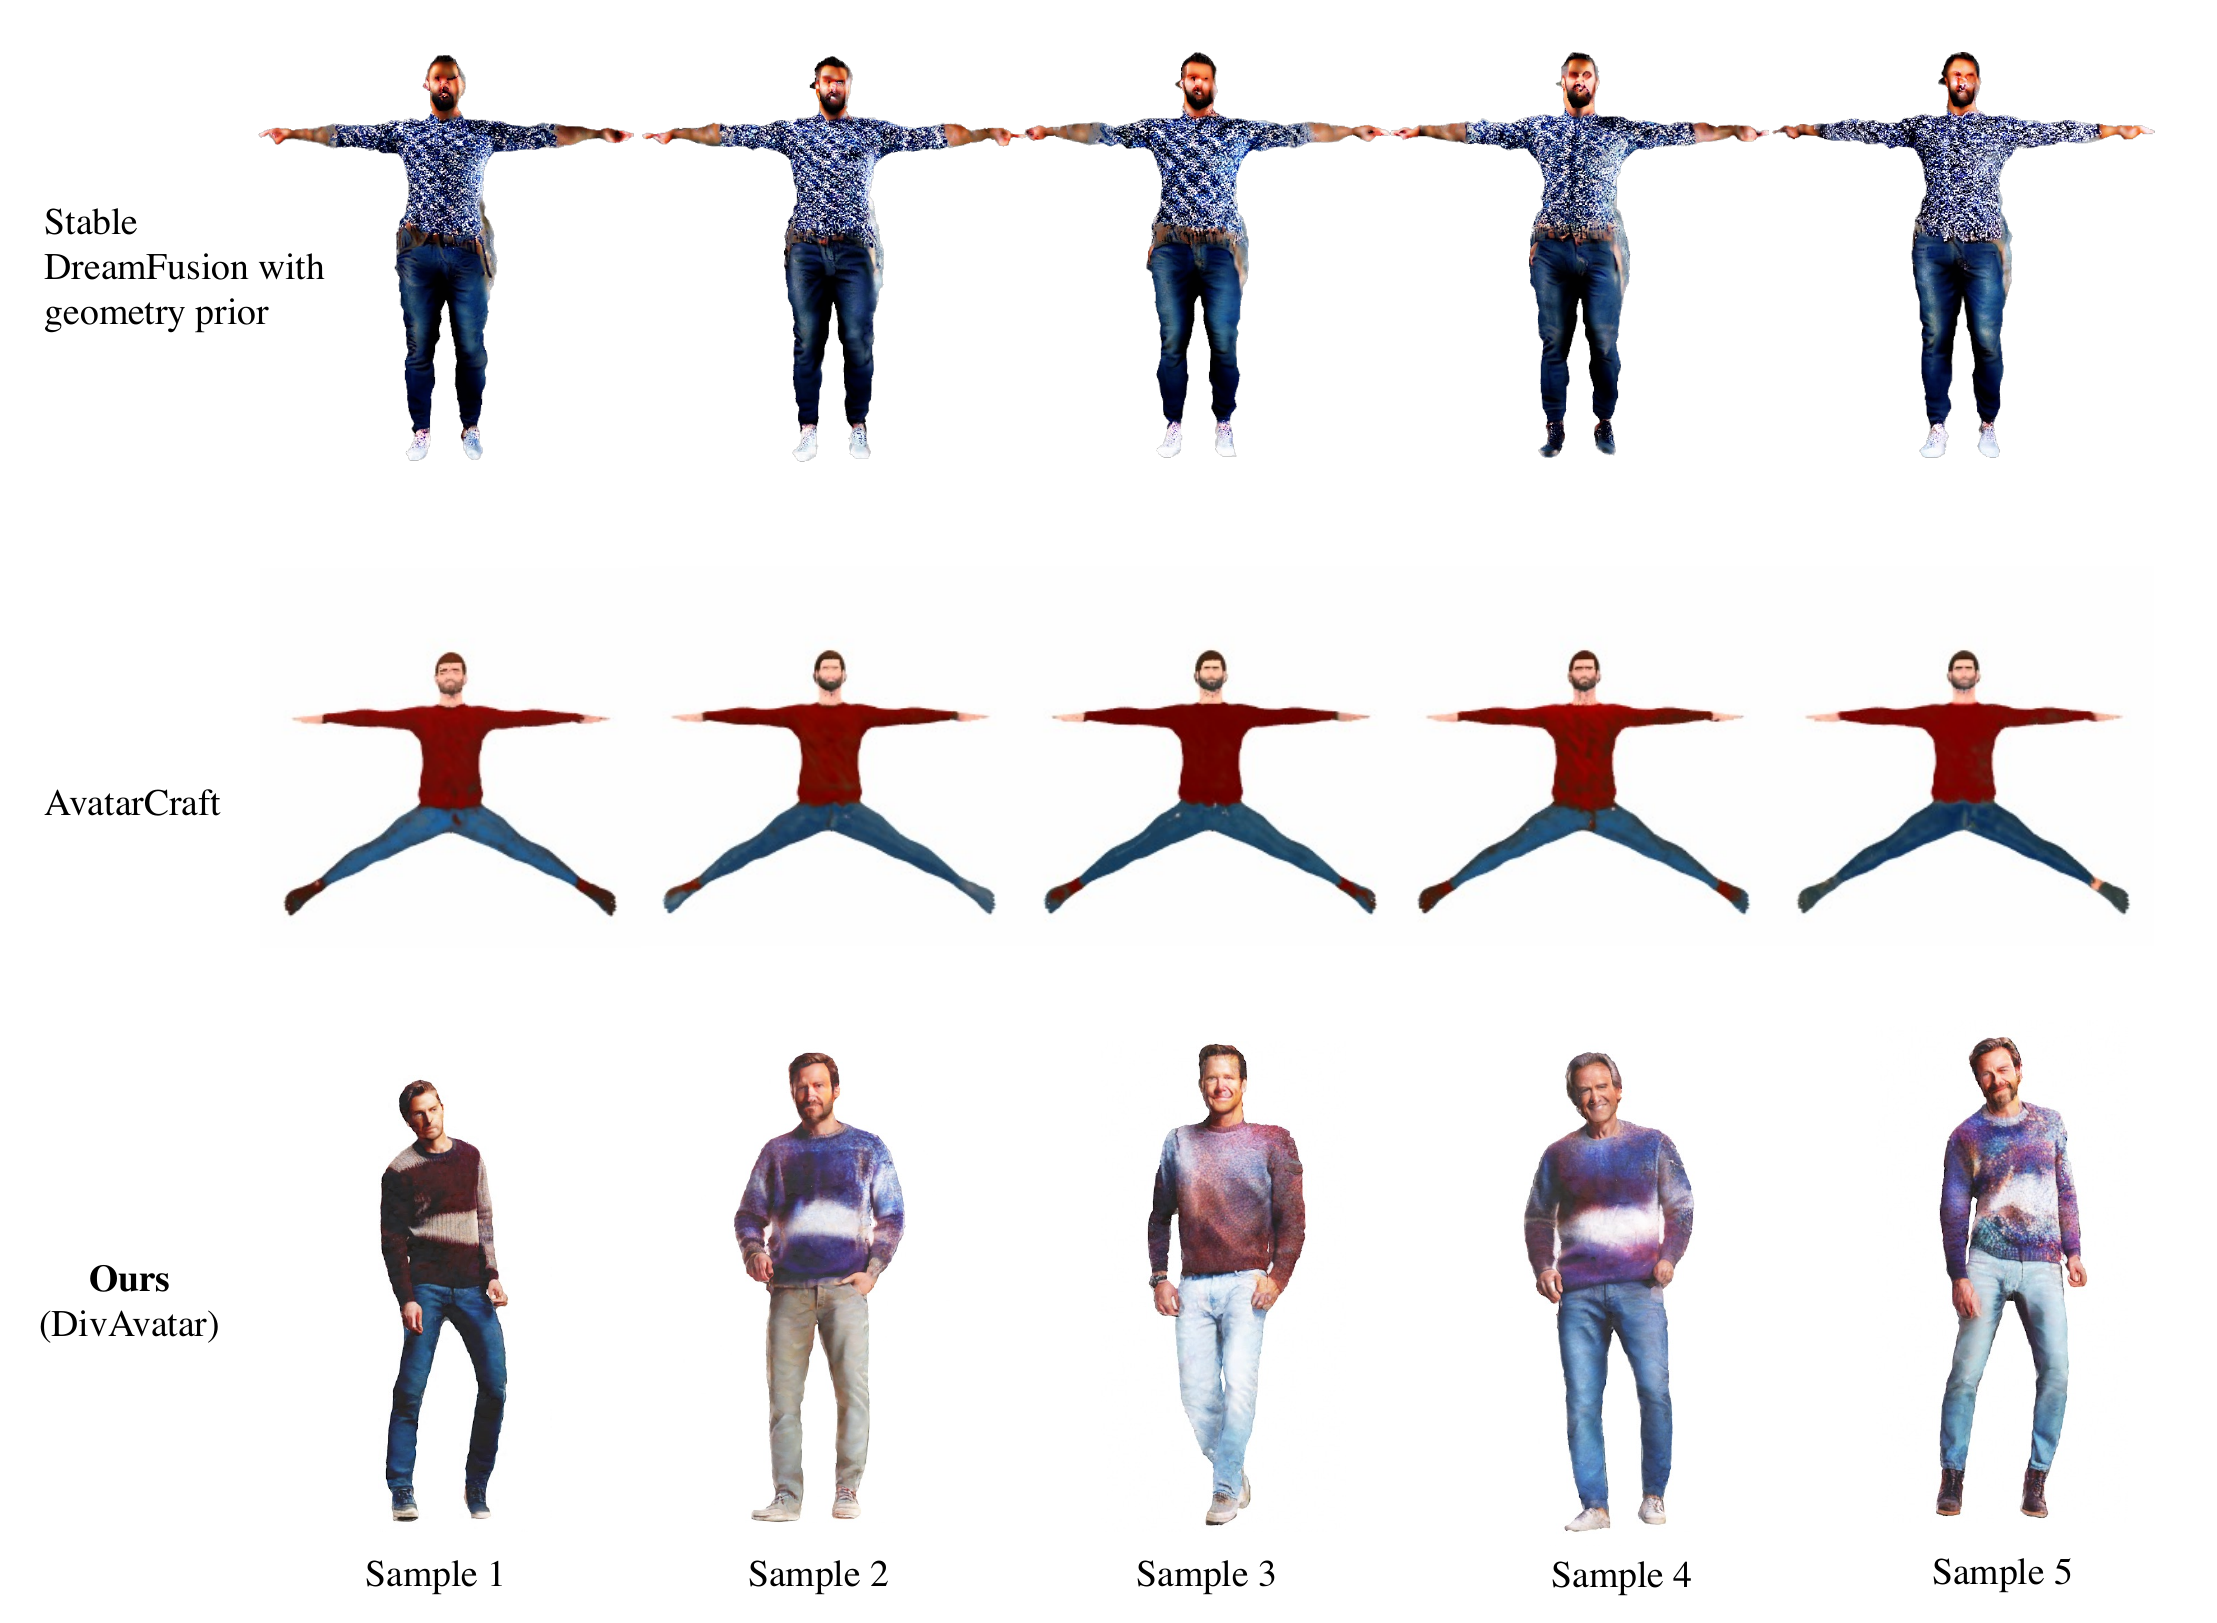}
   \caption{Input text prompt: \textit{A man wearing sweater and pants.}}
   \label{fig:sweater}
\end{figure*}

\begin{figure*}[h!]
  \centering
  % \fbox{\rule{0pt}{2in} \rule{0.9\linewidth}{0pt}}
   \includegraphics[width=0.8\linewidth]{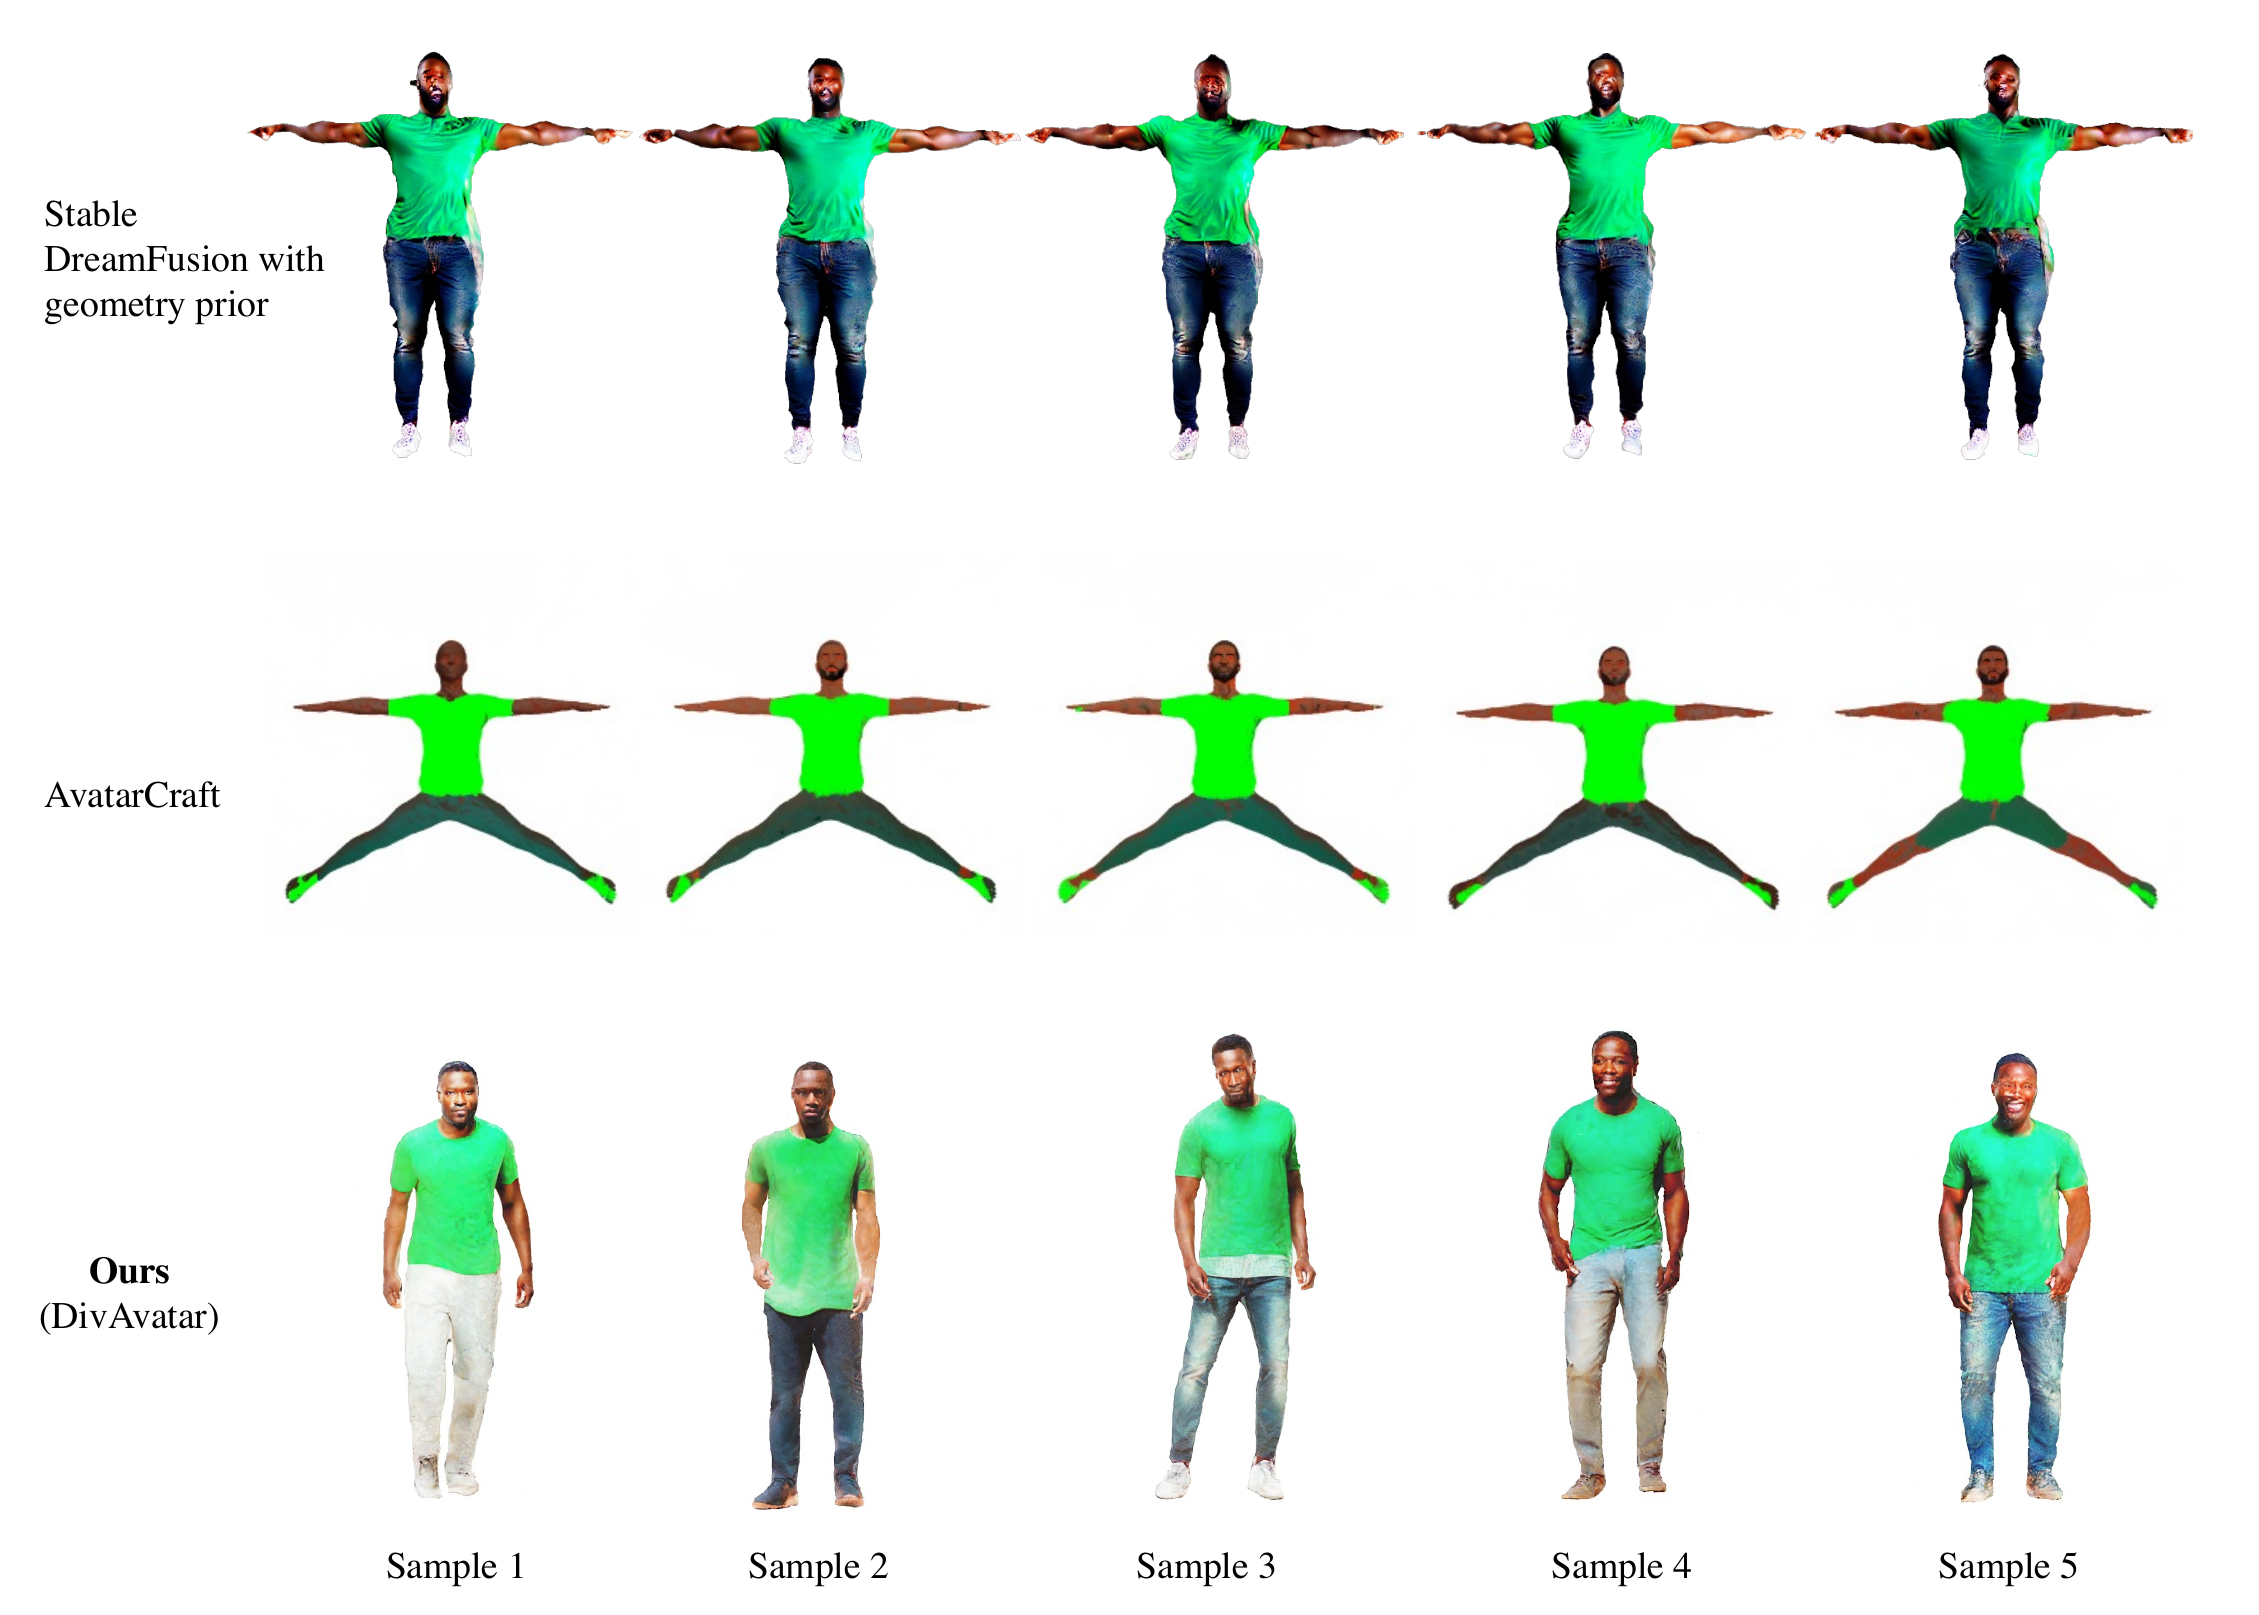}
   \caption{Input text prompt: \textit{A Black man wearing green tshirt.}}
   \label{fig:green5}
\end{figure*}

\begin{figure*}[h!]
  \centering
  % \fbox{\rule{0pt}{2in} \rule{0.9\linewidth}{0pt}}
   \includegraphics[width=0.8\linewidth]{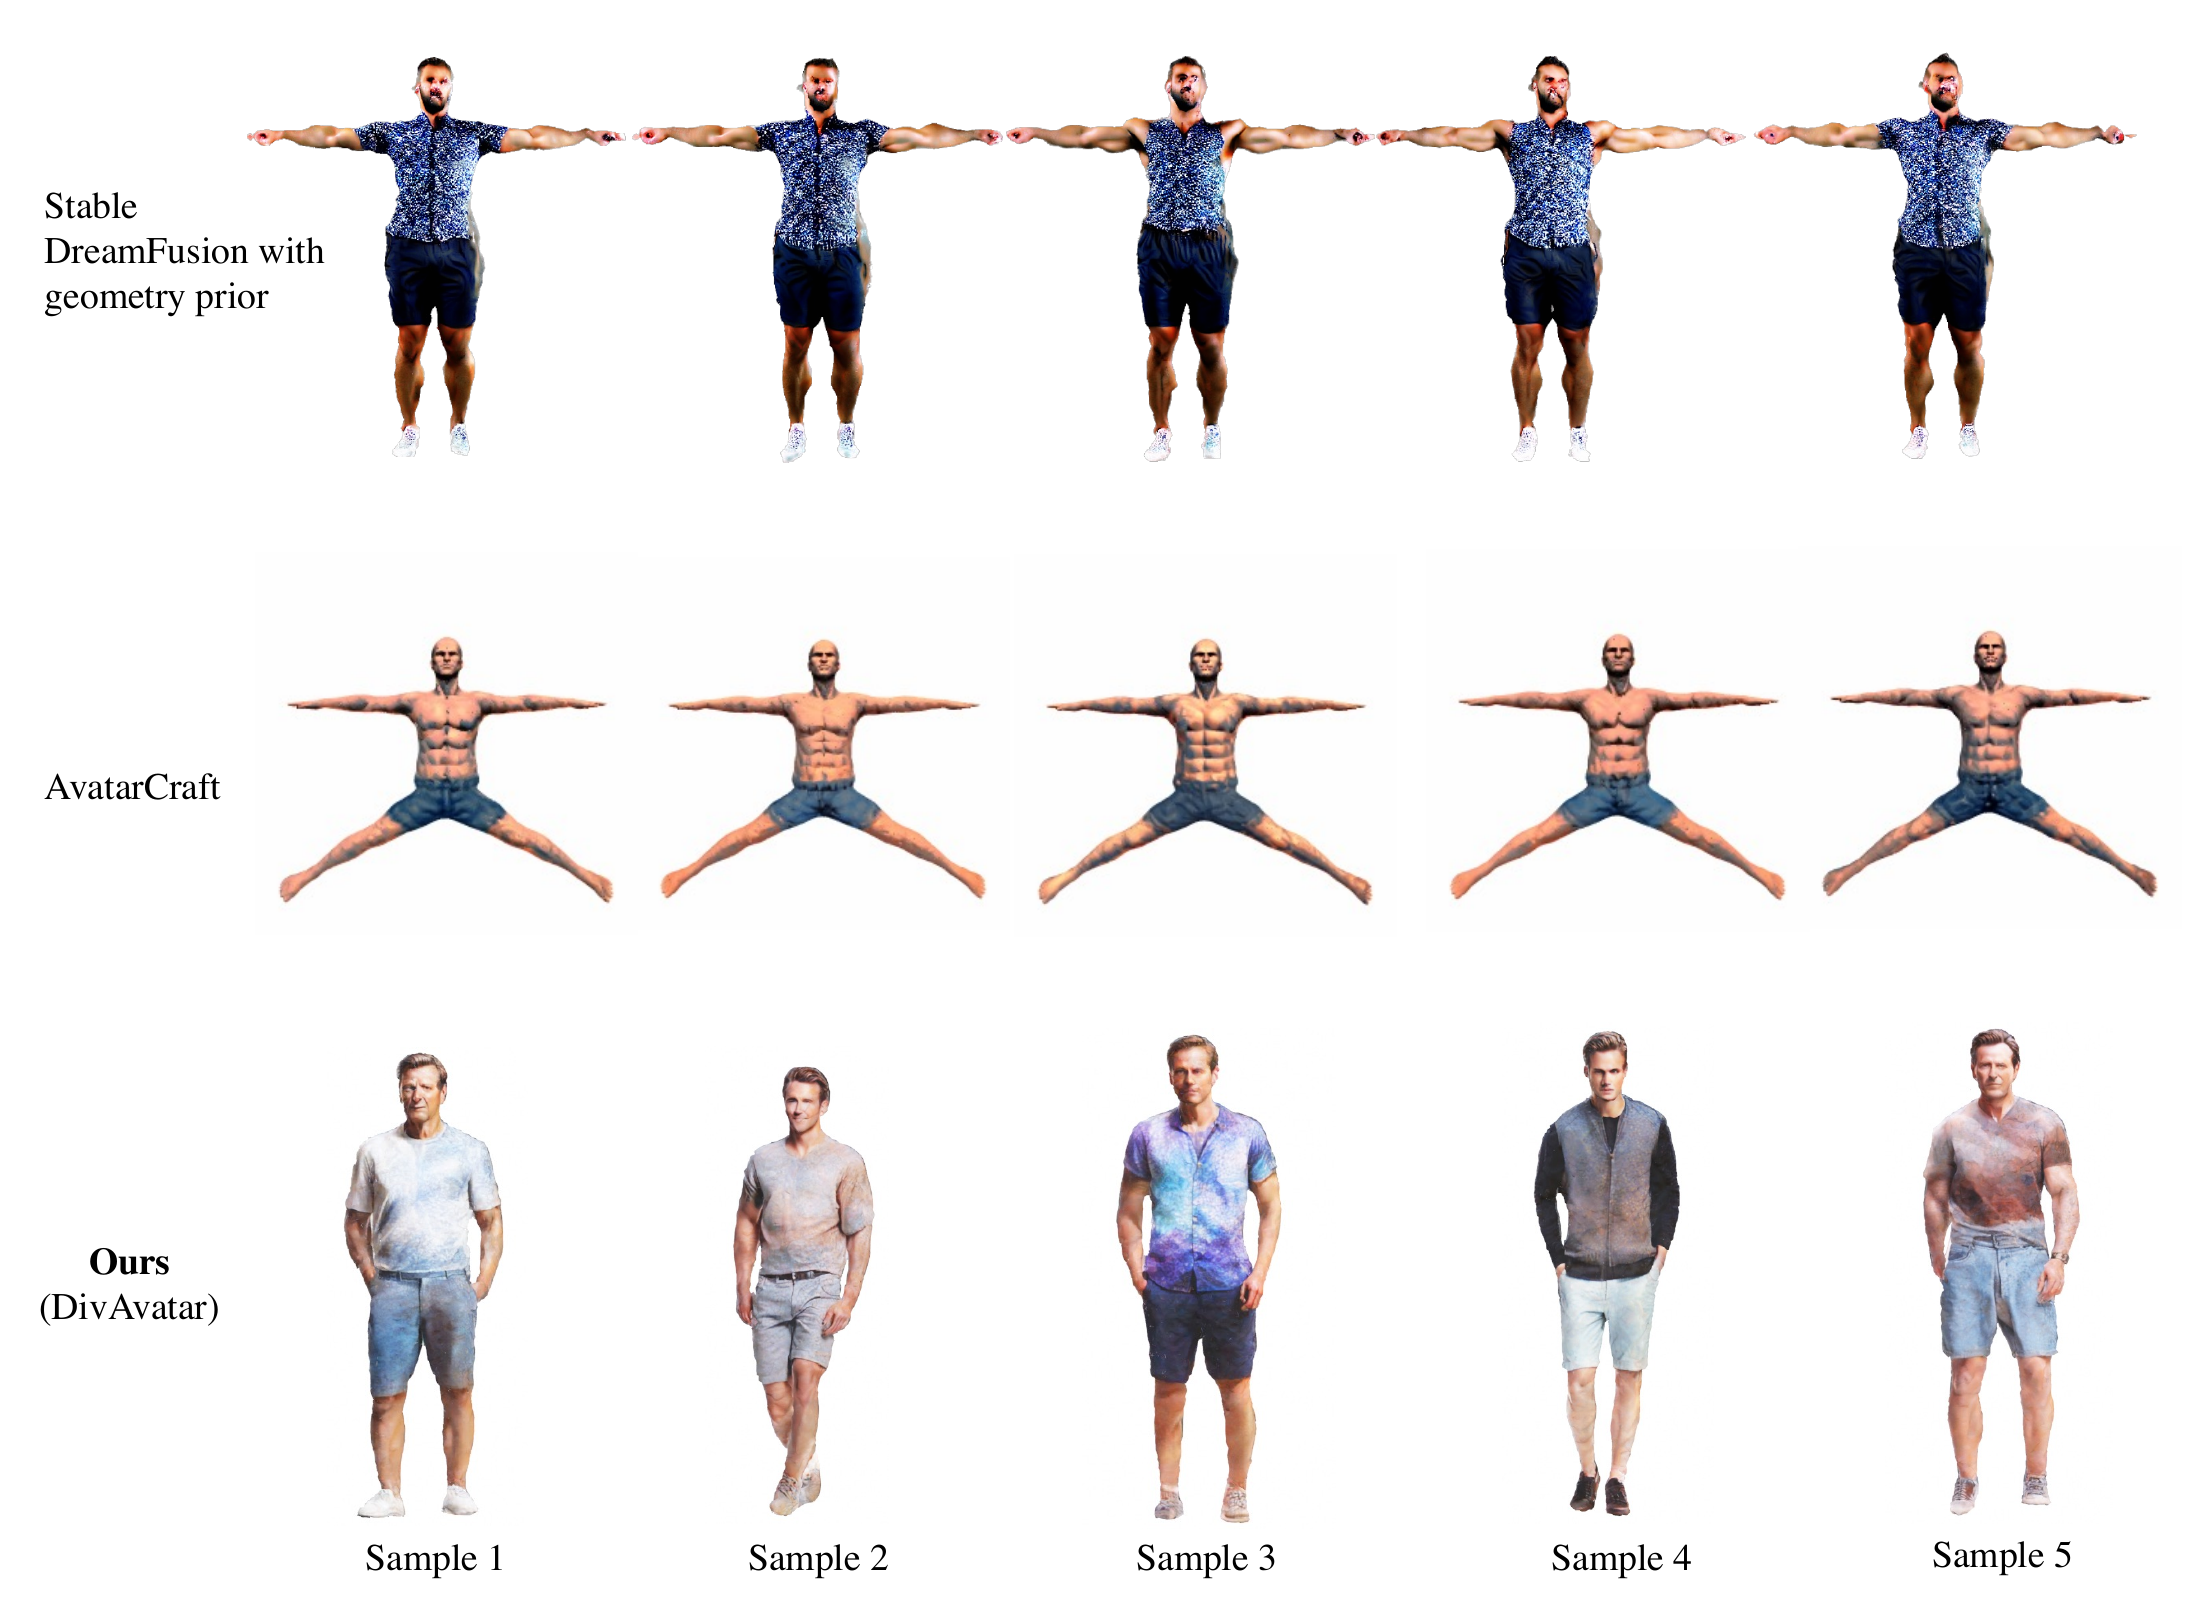}
   \caption{Input text prompt: \textit{A man wearing shorts.}}
   \label{fig:shorts}
\end{figure*}

\begin{figure*}[h!]
  \centering
  % \fbox{\rule{0pt}{2in} \rule{0.9\linewidth}{0pt}}
   \includegraphics[width=0.8\linewidth]{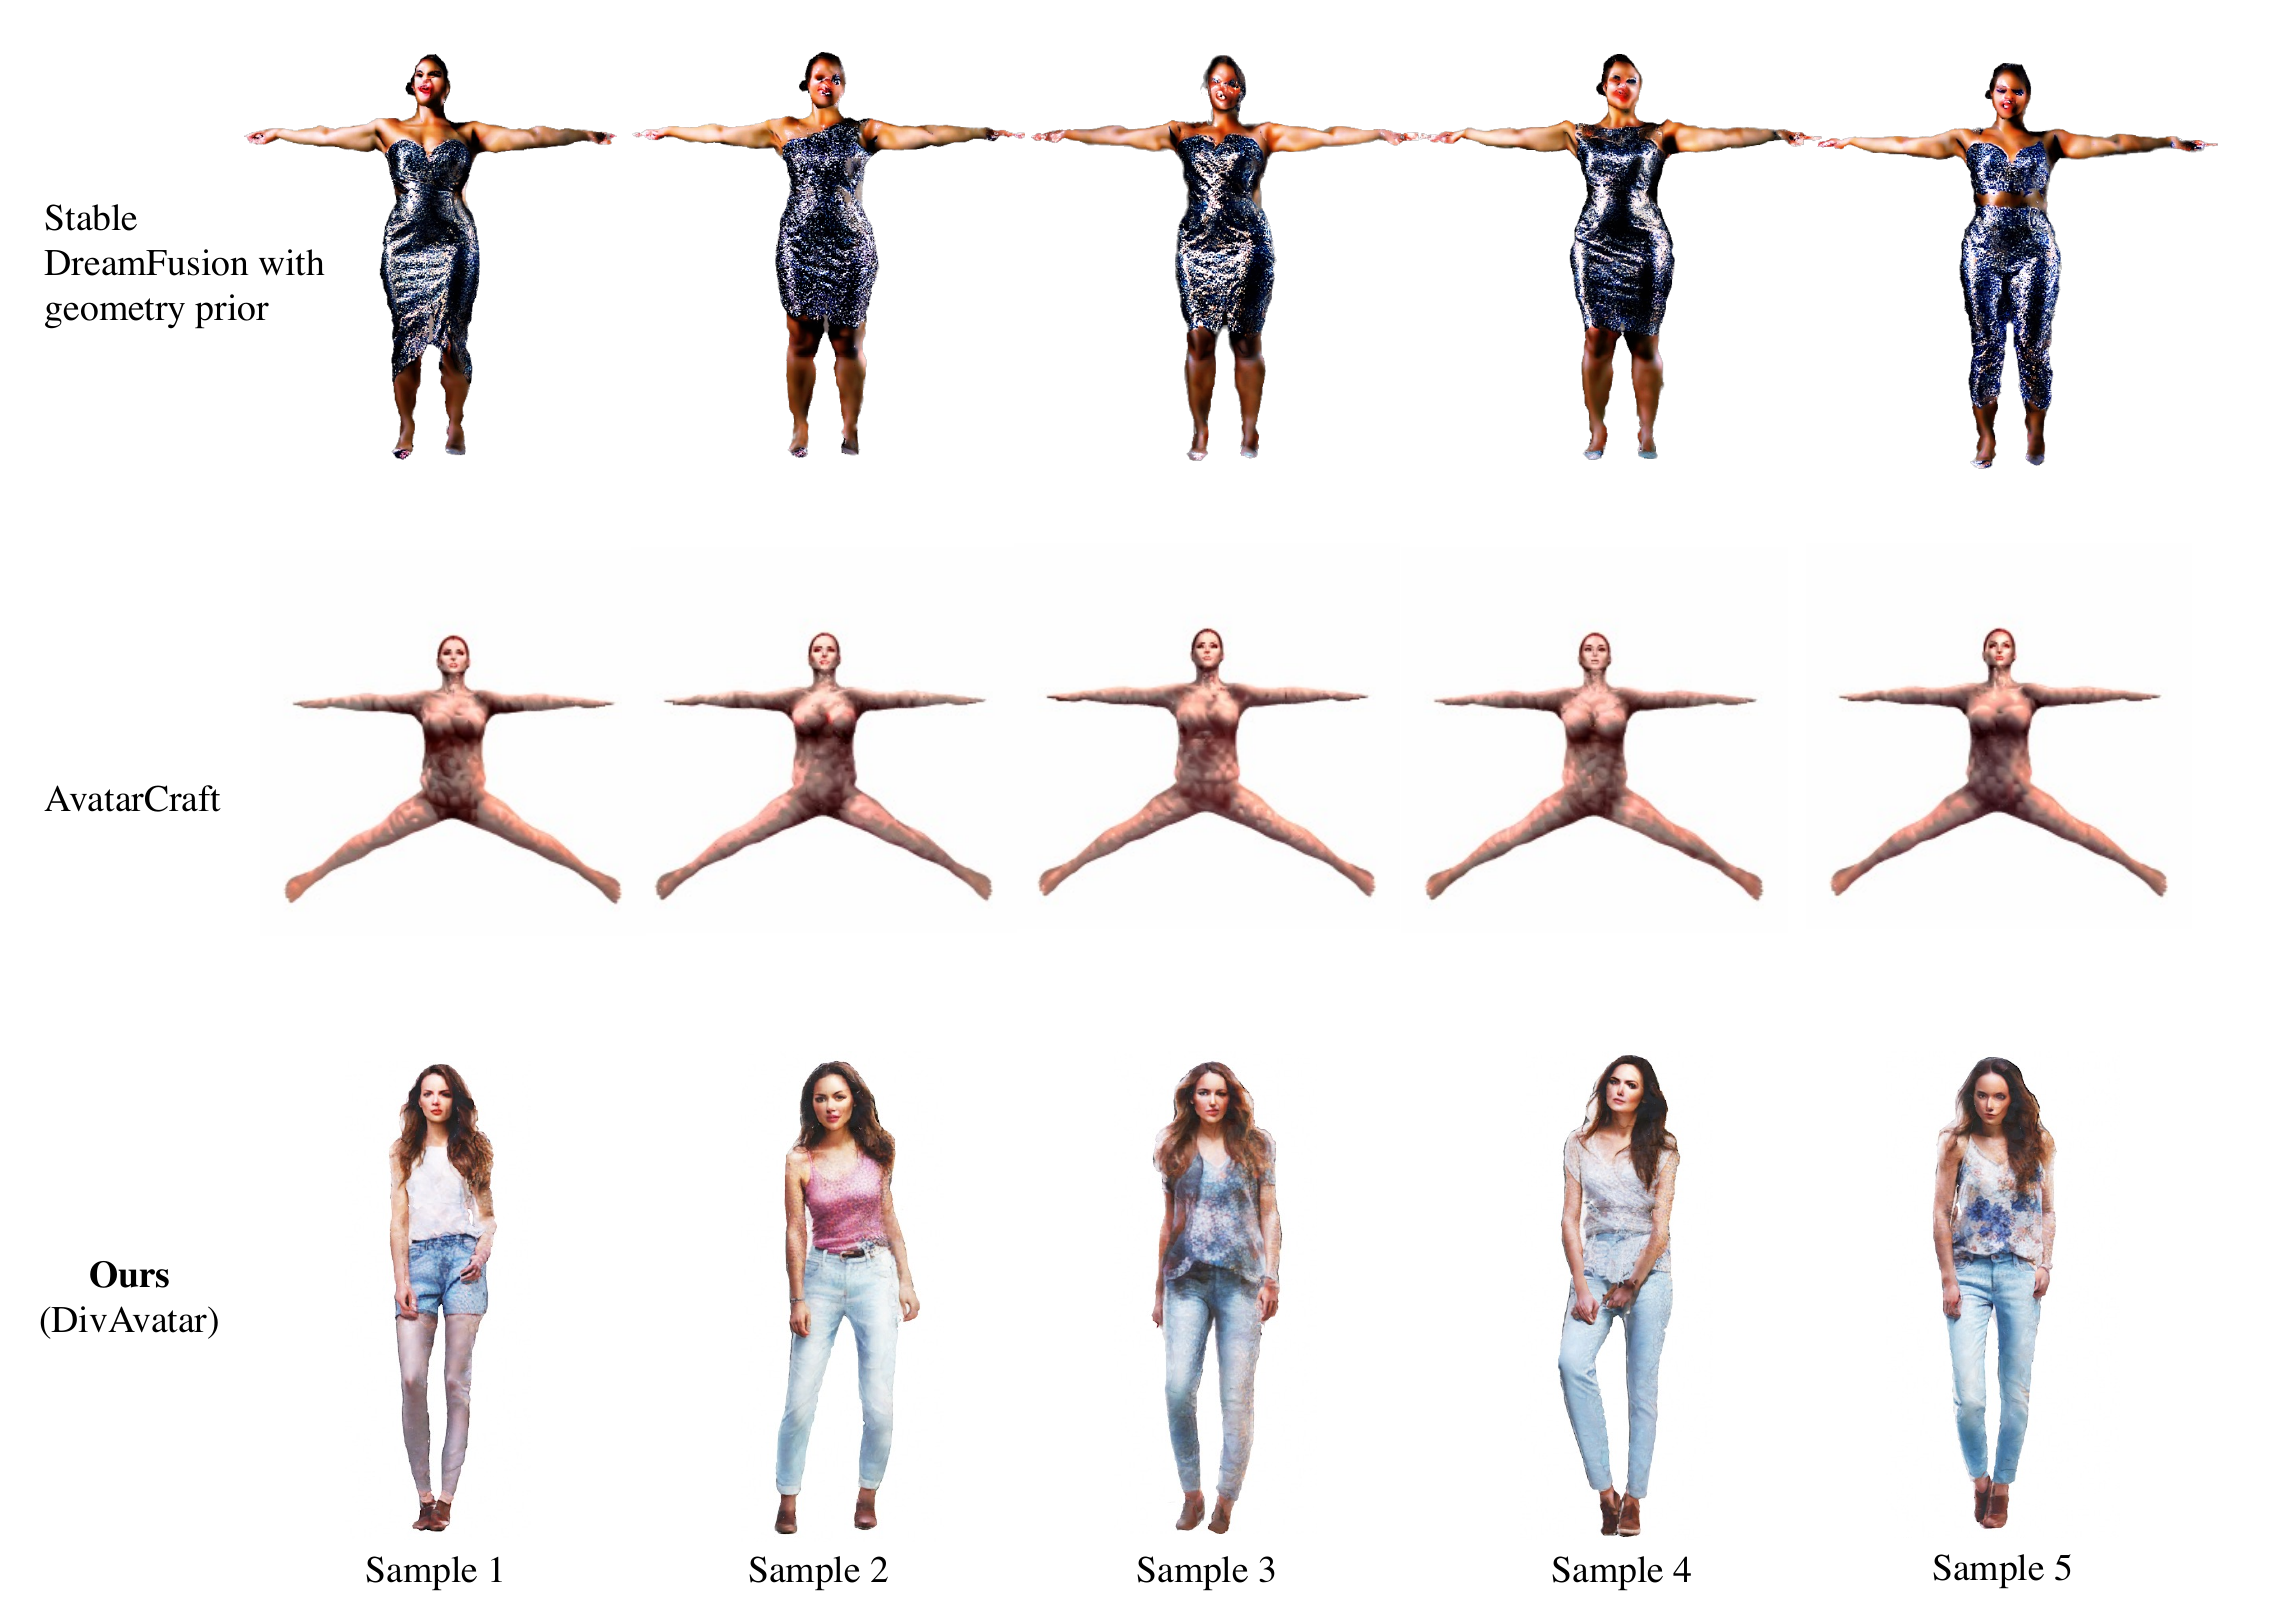}
   \caption{Input text prompt: \textit{A woman.}}
   \label{fig:woman}
\end{figure*}

% \begin{figure*}[h!]
%   \centering
%   % \fbox{\rule{0pt}{2in} \rule{0.9\linewidth}{0pt}}
%    \includegraphics[width=0.8\linewidth]{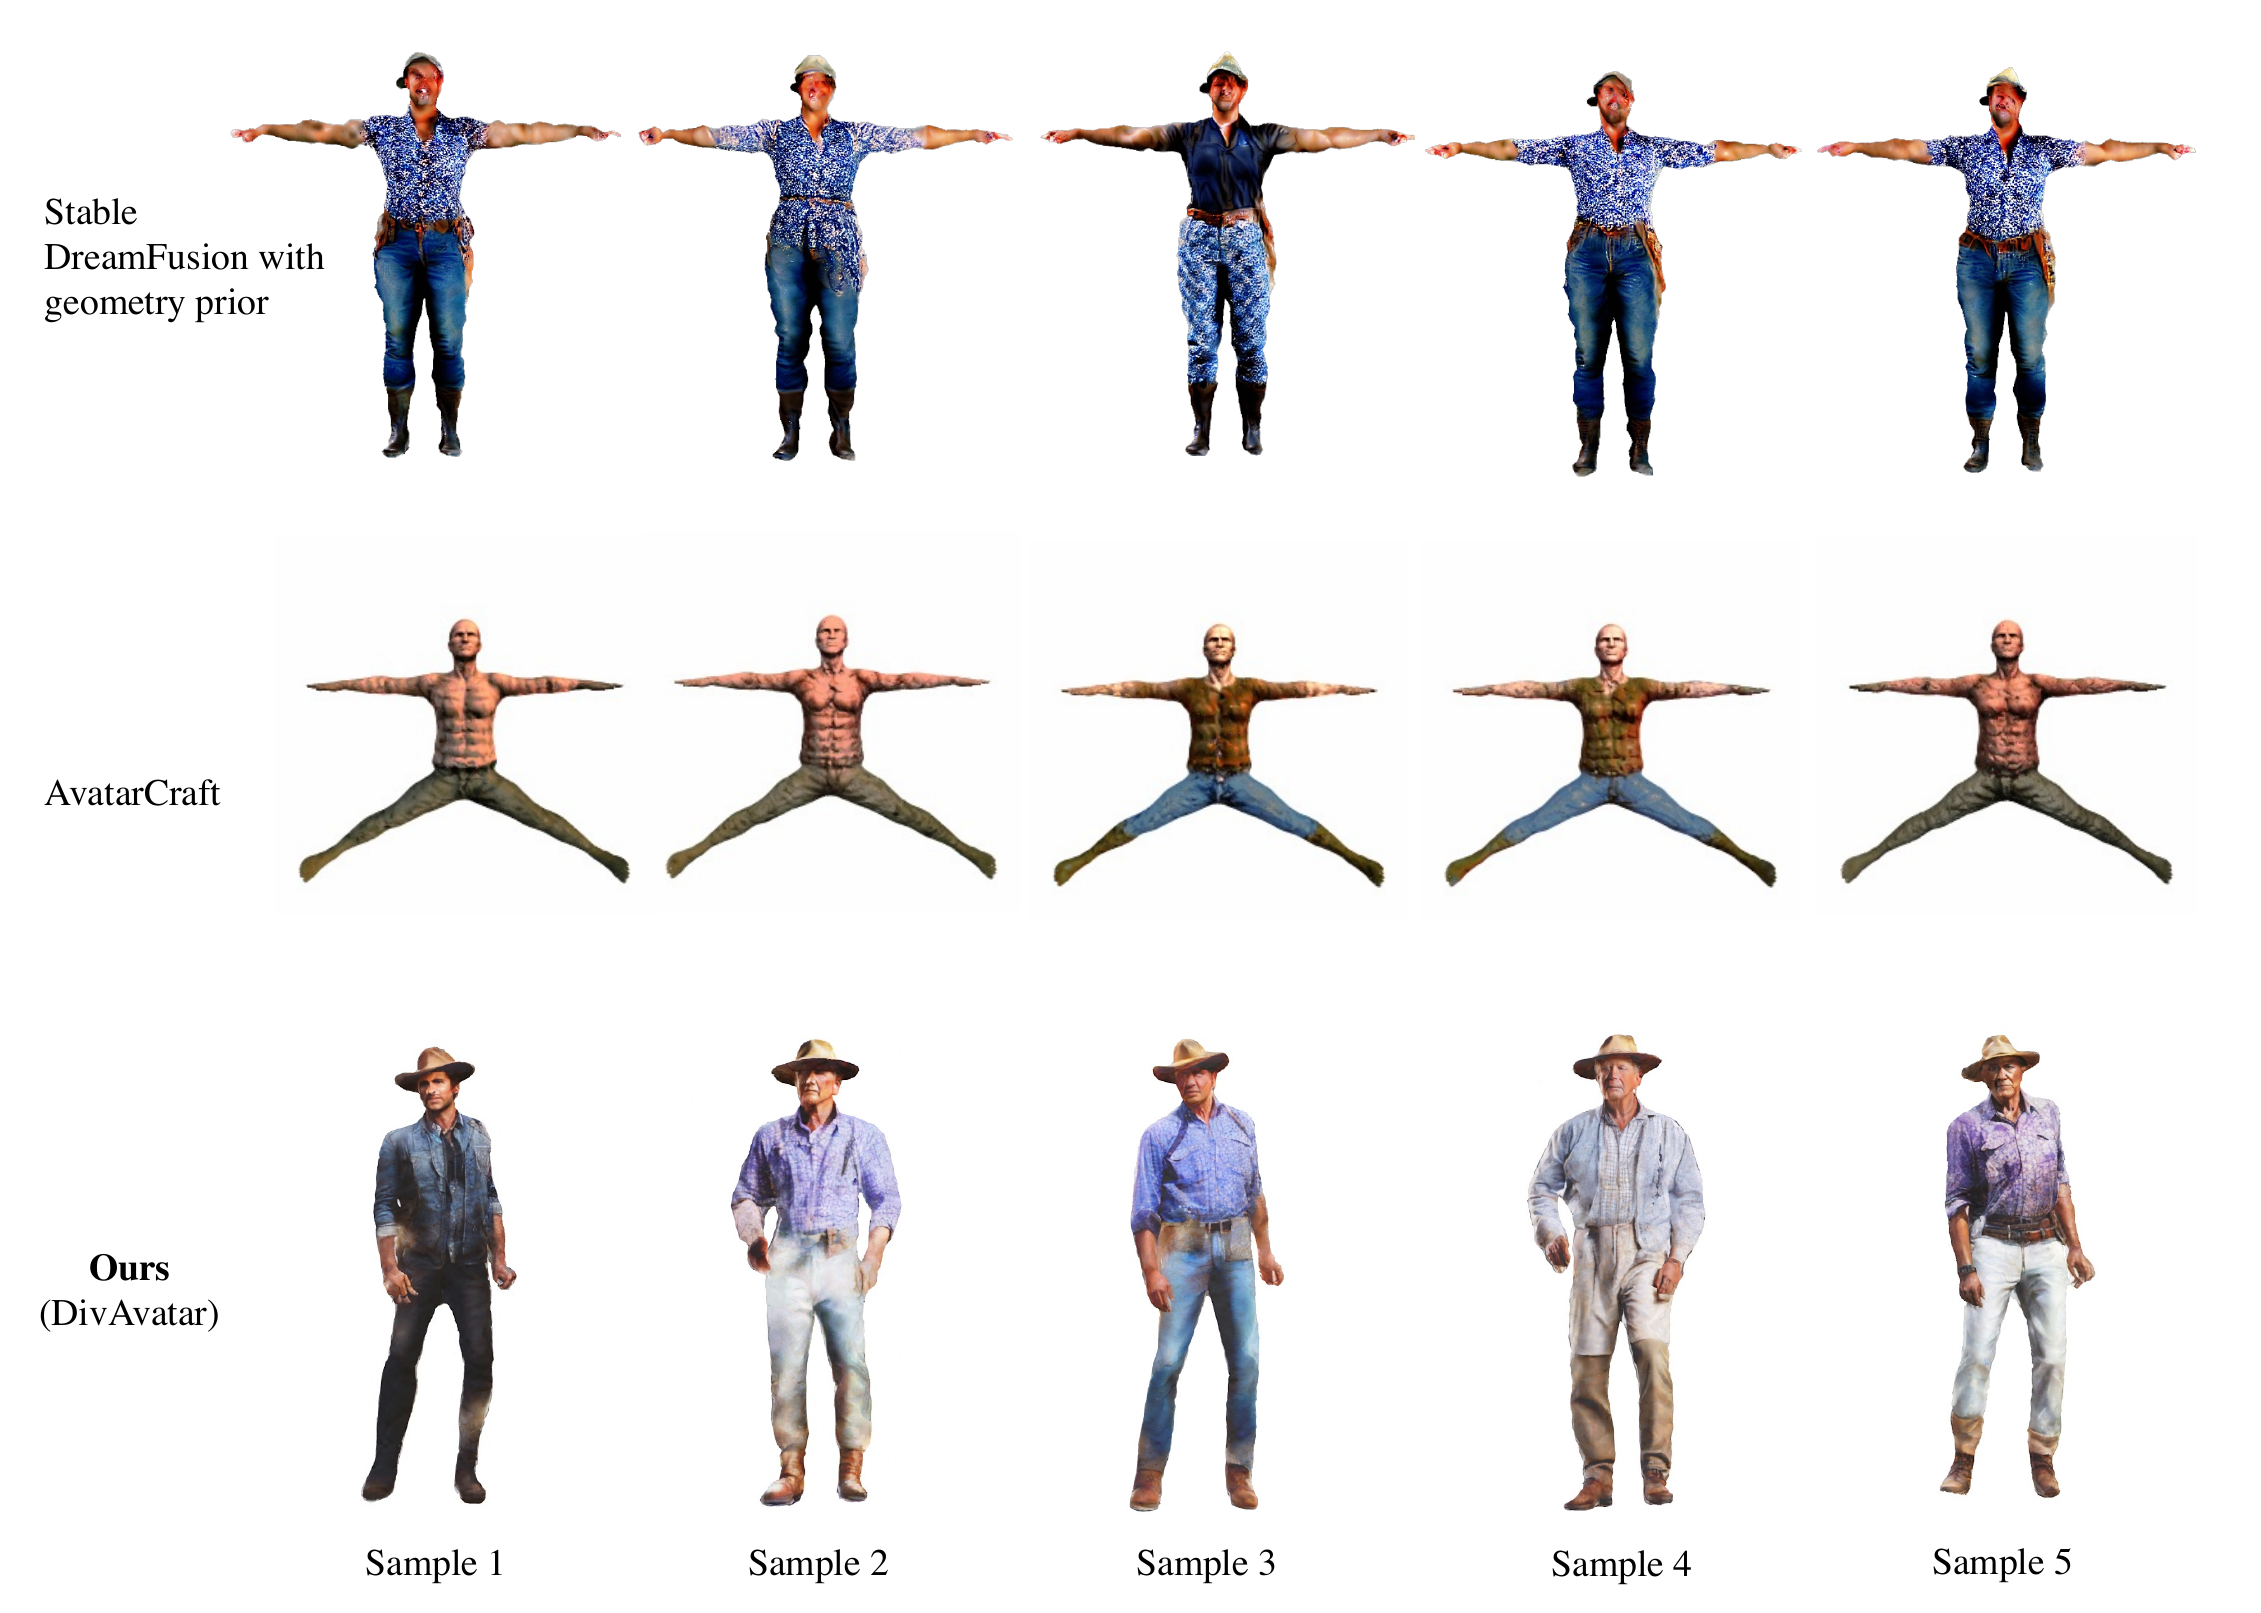}
%    \caption{Input text prompt: \textit{A farmer.}}
%    \label{fig:farmer5}
% \end{figure*}

\section{Implementation Details}
\label{sec:implementation}

In the process of finetuning the human generative model (EVA3D), we add the SDS loss and the feature-based depth loss to the generator only. The output rendering resolution of the human generative model is 512x256. We retrieve and pad the rendered front and back view of each generated human to 512x512 for img2img refinement \cite{img2img}. Interestingly, we found that the img2img refinement is able to generate front and back images that are consistent with each other. This consistency likely results from the multi-view consistency inherent in the input images used for the refinement process. 

We use the publicly available code \cite{stable-dreamfusion} for DMTet finetune, where the output rendered image is shape 1024x1024. To ensure that the diverse appearances from the finetuned generative model are not lost, we use the refined front and back images as image conditions. We alternate between SDS loss and the MSE loss at each iteration. We use the default value 1000 and 1 for MSE loss and SDS loss weights respectively.

The finetune of the human generative model process takes around 2 hours for one prompt, involving 5000 iterations. The inference process to obtain one sample is around 30 seconds. The mesh optimization process of each sample takes an average of 30 minutes involving img2img refinement and 5000 iterations of dmtet finetune.

% \section{User Study}

% We conduct user study to quantitatively assess our work's diversity by comparing our results with AvatarCraft and Stable Dreamfusion (as in our qualitative comparisons). We select 6 sets of generated outcomes of different text prompts. One set of result contains five samples from AvatarCraft, Stable Dreamfusion, and DivAvatar each. A total of 36 participants were involved in the user studies to vote for their most preferred results based on diversity, quality and text alignment for each set. We present our quantitative results in \cref{tab:quantitative_results}. The user preference percentage is calculated by summing the total user choice for each method in each aspect across the 6 sets of results. The results demonstrate that our method achieves significantly superior preference over the comparative methods, particularly in diversity.

% \begin{table}[h!]
% \centering
% \begin{tabular}{p{2cm}p{1.5cm}p{1.5cm}p{1.6cm}}\hline
% \toprule
% & \textbf{Diversity} & \textbf{Image Quality} & \textbf{Text Alignment} \\
% \midrule
% S.D & 1.8 & 4.6 & 11.6 \\
% AvatarCraft       & 0.4 & 1.0 & 5.5 \\
% Ours              & \textbf{97.8} & \textbf{94.4} & \textbf{82.9} \\
% \bottomrule
% \end{tabular}
% \caption{Quantitative results of user study. We compare with Stable Dreamfusion (abbreviated as S.D) and AvatarCraft in three aspects: 1) Diversity, 2) Image Quality, and 3) Text Alignment. The table shows the user preference in percentage.}
% \label{tab:quantitative_results}
% \end{table}
